# Supplementary material for: Computing total progeny distributions of multi-type Galton--Watson processes
Source: arXiv:2606.03007 source file (2026-12-01)
Supplement: Supplementary file 1 [file okada_aoas_supp_submit.tex]

\documentclass[aoas]{imsart}

%% Packages
\RequirePackage{amsthm,amsmath,amsfonts,amssymb}
\RequirePackage[authoryear]{natbib}
\RequirePackage{bm}
\RequirePackage{mathtools}
\RequirePackage{graphicx}

\startlocaldefs
\numberwithin{equation}{section}

\theoremstyle{plain}

\theoremstyle{definition}

\endlocaldefs

\begin{document}

\begin{frontmatter}
\title{Supplementary material for ``Computing the final epidemic size distributions of a multi-type Galton--Watson process''}
\runtitle{Supplementary material}

\begin{aug}
\author[A]{\fnms{Yuta}~\snm{Okada}\ead[label=e1]{okada.yuta.4y@kyoto-u.ac.jp}}
\and
\author[A]{\fnms{Hiroshi}~\snm{Nishiura}\ead[label=e2]{nishiura.hiroshi.5r@kyoto-u.ac.jp}}

\address[A]{School of Public Health, Graduate School of Medicine, Kyoto University\printead[presep={,\ }]{e1,e2}}
\end{aug}

\end{frontmatter}

\section{Proof of Proposition 3.1}Restatement of Proposition 3.1:

Let $\bm{G}(\bm{z} )=(G^{(1)}(\bm{z}),...,G^{(n)}(\bm{z}))^{T}$ be the offspring probability generating function (PGF) vector
of an $n$-type Galton--Watson process (GWP) defined for $|z_{i}|\le1$, $i=1,2,...,n$, such that
$\bm{J}_{\bm{G}}(\bm{r})$ has finite elements and is nonnegative and irreducible for $\bm r \in (0, 1]^n$.
Then, there exists $\bm{r}^{\#}=(r_{1}^{\#},...,r_{n}^{\#}) \in [0,1]^n$ such that, for every complex
vector $\bm{z}$ inside the polydisk $D_{\bm{z}}:|z_{i}|<r_{i}^{\#}$, $i=1,...,n$, the functional equation
\[
\bm{h} =  \operatorname{diag}(\bm{z})\bm{G}(\bm{h}) \eqqcolon \bm{T}_{\bm{z}}(\bm{h})
\]
has a unique solution $\bm{h}\in\mathbb{C}^{n}$ with $|\bm {h}|\leq |\bm z| <\bm{r}^{\#}$.

\begin{proof}
First, by definition, the elements of both $\bm{G}$  and its Jacobian matrix $\bm{J}_{\bm{G}}(\bm{z})=\left[ \left(\frac{\partial G^{(i)}}{\partial z_j} \right)_{i,j} \right] \in \mathbb{C}^{n \times n}$ are multivariate power series with nonnegative coefficients. Therefore, the following relationship holds for the weighted infinity norm by an arbitrary positive vector $\bm{x}$:
\begin{equation}
\label{eq:norm_ineq}
\|\bm{J}_{\bm{G}}(\bm{z})\|_{\infty,\bm{x}} \le \| |\bm{J}_{\bm{G}}(\bm{z})| \|_{\infty,\bm{x}} \le \|\bm{J}_{\bm{G}}(|\bm{z}|)\|_{\infty,\bm{x}},
\end{equation}
where $\|\bm{A}\|_{\infty,\bm{x}}=\max_{i}(\frac{(|\bm{A}|\bm{x})_{i}}{x_{i}})$. (Hereafter, we denote $|\bm{z}|=\bm{r}\in\mathbb{R}^{n}$.) Because $\bm{J}_{\bm{G}}(\bm{r})$ is nonnegative and irreducible, the Perron--Frobenius theorem implies that $\bm{J}_{\bm{G}}(\bm{r})$ has positive left and right leading eigenvectors $\bm{u}(\bm{r})$ and $\bm{v}(\bm{r})$ for every $\bm{r}=(r_{1},...,r_{n})$, $r_{i}\in(0,1]$ (for simplicity, we assume $\bm{u}^{T}\bm{v}=1$ without loss of generality) \citep{hornjohnson2012matrix}. The elements of $\bm{J}_{\bm{G}}(\bm{r})$ and $\rho(\bm{J}_{\bm{G}}(\bm{r}))$, and the spectral radius of $\bm{J}_{\bm{G}}(\bm{r})$, are nondecreasing functions of $\bm{r}$.

Next, regarding  $\bm{T}_{\bm{z}}(\bm{h})$, it readily follows that $|\bm{T}_{\bm{z}}(\bm{h})|<|\bm{z}|=\bm{r}\le \bm{1}$ when $|\bm{h}|\le|\bm{z}|=\bm{r}\le\bm{1}$. Suppose we have $\bm{h}, \bm{h}^{\prime}$ such that $\bm{h}\ne \bm{h}^{\prime}$ and $|\bm{h}|\le|\bm{z}|,|\bm{h}^{\prime}|\le|\bm{z}|$. Here, we consider a linear path $\bm{\omega}(t)=\bm{h}+t(\bm{h}^{\prime}-\bm{h})$, $t\in[0,1]$. Note that  $|\bm{\omega}(t)|\le \max(|\bm{h}|,|\bm{h}^{\prime}|)=\bm{r}$ and $|\bm{T}_{\bm{z}}(\bm{\omega}(t))|<|\bm{z}|\le \bm{1}$. By writing  $\bm{G}(\bm{h}^{\prime})-\bm{G}(\bm{h})$ in the integral form as
\begin{equation}
\bm{G}(\bm{h}^{\prime})-\bm{G}(\bm{h})=\int_{t=0}^{t=1}\bm{J}_{\bm{G}}(\bm{\omega}(t))(\bm{h}^{\prime}-\bm{h})dt,
\end{equation}
Eq.~\eqref{eq:norm_ineq} implies that the following relationship holds for an infinity norm weighted by an arbitrary positive vector $\bm{x}$:
\begin{align}
\|\bm{G}(\bm{h}^{\prime})-\bm{G}(\bm{h})\|_{\infty,\bm{x}} & \le \|\int_{t=0}^{t=1}\bm{J}_{\bm{G}}(\bm{\omega}(t))(\bm{h}^{\prime}-\bm{h})dt\|_{\infty,\bm{x}} \notag \\
&\le \|\int_{t=0}^{t=1}\bm{J}_{\bm{G}}(|\bm{\omega}(t)|)\|_{\infty,\bm{x}}\|\bm{h}^{\prime}-\bm{h}\|_{\infty,\bm{x}} dt\notag \\
&\le \|\bm{J}_{\bm{G}}(\max(|\bm{h}|,|\bm{h}^{\prime}|))\|_{\infty,\bm{x}}\|\bm{h}^{\prime}-\bm{h}\|_{\infty,\bm{x}} \notag \\
&\le \|\bm{J}_{\bm{G}}(\bm{r})\|_{\infty,\bm{x}}\|\bm{h}^{\prime}-\bm{h}\|_{\infty,\bm{x}}.
\end{align}
Thus, it follows that
\begin{equation}
\|\bm{T}_{\bm{z}}(\bm{h}^{\prime})-\bm{T}_{\bm{z}}(\bm{h})\|_{\infty,\bm{x}}\le \|\operatorname{diag}(\bm r)\bm{J}_{\bm{G}}(\bm{r})\|_{\infty,\bm{x}}.\|\bm{h}^{\prime}-\bm{h}\|_{\infty,\bm{x}}.
\end{equation}

Setting $\bm M(\bm r) = \operatorname{diag}(\bm r)\bm{J}_{\bm{G}}(\bm{r})$, we now show the existence of $\bm{r}^{\#} \in \mathbb{R}^n$ and $\bm x = \bm{x}(\bm r^{\#})\in \mathbb{R}^n$ such that $\| \bm M(\bm r^{\#})  \|_{\infty, \bm x}<1$ regardless of the criticality of $\bm{G}$. 

(i) Subcritical case: $\rho(\bm{J}_{\bm{G}}(\bm{1}))<1$.
It can be seen that $\rho(\bm M(\bm r ))<1$ for all $\bm r \in [0, 1]^n$, because $\bm M(\bm r ) \leq \bm{J}_{\bm{G}}(\bm{r}) \leq \bm{J}_{\bm{G}}(\bm{1})$ holds element-wise. Therefore, by letting $\bm x(\bm r) = \bm v$ be the leading right eigenvector of $\bm M(\bm r)$, $\| \bm M(\bm r)  \|_{\infty, \bm v} = \rho(\bm M(\bm r) )<1$.

(ii) Critical case: $\rho(\bm{J}_{\bm{G}}(\bm{1}))=1$.
The same discussion as in (i) holds for all $\bm{r}\in [0, 1-\epsilon]^n$.

(iii) Supercritical case: $\rho(\bm{J}_{\bm{G}}(\bm{1}))>1$.
The vector of extinction probabilities $\bm{q}=(q_{1},q_{2},...,q_{n})\in[0,1)^{n}$ is the minimum real-valued solution of $\bm{q}=\bm{G}(\bm{q})$, and $\rho(\bm{J}_{\bm{G}}(\bm{q}))<1$. Here, for simplicity, we consider a linear path from $\bm{q}$ to $\bm{1}$, $\bm{r}(t)=\bm{q}+t(\bm{1}-\bm{q})$,  $t\in[0,1]$. 
Because $\rho(\bm M(\bm r(0) ))=\rho(\bm M(\bm q))<1$ and $\rho(\bm M(\bm r(1) )) =\rho(\bm{J}_{\bm{G}}(\bm{1}))>1 $, there exist $t^{*} \in [0, 1]$ such that $\rho(\bm M(\bm r(t^{*}) ))=1$. Therefore, by choosing $\bm r = \bm r(t^{*}-\epsilon)$, it again follows that $\| \bm M(\bm r)  \|_{\infty, \bm v} = \rho(\bm M(\bm r) )<1$.

The discussion in (i)--(iii) ensures the existence of $\bm{r}^{\#}$ and $\bm{x} = \bm v(\bm r^{\#})$ such that $\| \bm M(\bm r)  \|_{\infty, \bm x}<1$. Therefore, the following holds for two vectors $\bm{h}$ and $\bm{h}^{\prime}$ satisfying $|\bm{h}|\le|\bm{z}|,|\bm{h}^{\prime}|\le|\bm{z}|$:
\begin{equation}
\label{eq:Tz_lipconst}
\|\bm{T}_{\bm{z}}(\bm{h}^{\prime})-\bm{T}_{\bm{z}}(\bm{h})\|_{\infty,\bm{v}(\bm{r}^{\#})}\le L\|\bm{h}^{\prime}-\bm{h}\|_{\infty,\bm{v}(\bm{r}^{\#})},
\end{equation}
where $L=\| \bm M(\bm r)  \|_{\infty, \bm v(\bm r^{\#})}<1$. Equation \eqref{eq:Tz_lipconst} ensures that, for a sequence $\bm{h}^{\{k\}}$ defined by $\bm{h}^{\{k+1\}}=\bm{T}_{\bm{z}}(\bm{h}^{\{k\}})$, $\bm{h}^{\{0\}}\le|\bm{z}|<\bm{r}^{\#}$, it follows that $\|\bm{h}^{\{k+1\}}-\bm{h}^{\{k\}}\|_{\infty,\bm{v}(\bm{r}^{\#})}$ decreases geometrically as $k\rightarrow\infty$, ensuring the existence of $\lim_{k\rightarrow\infty}\bm{h}^{\{k\}}=\bm{h}^{\{\infty\}}$,  the solution to the fixed-point equation \(\bm{h} = \operatorname{diag}(\bm{z})\bm{G}(\bm{h})\). 
Equation \eqref{eq:Tz_lipconst} also implies that $\bm{h}^{\{\infty\}}$ must be a unique solution. If two distinct vectors $\bm{h}^{\prime}$ and $\bm{h}^{\prime  \prime}$ satisfying $|\bm{h}^{ \prime}|\le|\bm{z}|,|\bm{h}^{\prime  \prime}|\le|\bm{z}|$ are the solutions to $\bm{h} =  \bm{T}_{\bm{z}}(\bm{h})$, applying $\bm{T}_{\bm{z}}$ to both vectors leads to
\begin{equation}
\|\bm{h}^{\prime  \prime}-\bm{h}^{ \prime} \|_{\infty,\bm{v}(\bm{r}^{\#})}=\|\bm{T}_{\bm{z}}(\bm{h}^{\prime  \prime})-\bm{T}_{\bm{z}}(\bm{h}^{ \prime})\|_{\infty,\bm{v}(\bm{r}^{\#})}\le L\|\bm{h}^{\prime  \prime}-\bm{h}^{ \prime}\|_{\infty,\bm{v}(\bm{r}^{\#})},
\end{equation}
which can only happen when $\bm{h}^{\prime  \prime}=\bm{h}^{ \prime}$. Thus, there exists $\bm{r}^{\#}$ such that a unique solution exists in $|\bm{h}|\le|\bm{z}|<\bm{r}^{\#}$ for $\bm{h} = \bm{T}_{\bm{z}}(\bm{h})$.
\end{proof}

\section{Connection between the existence of derivatives and the choice of contour}
\label{supp:higher_deriv_existence}

As mentioned in the main text, the argument presented in the proof of Proposition 3.1 is essentially equivalent to choosing a domain for $\bm z$ in which the derivatives of $\bm H(\bm z)$ are finite. 

Under the usual assumptions of Proposition 3.1, the derivatives of $\bm G(\bm z)$ are analytic in $|\bm z|< \bm r^{\#}$. Implicit differentiation of $\bm{H}(\bm{z}) = \operatorname{diag}(\bm{z})\bm{G}(\bm{H}(\bm{z}))$ with respect to $\bm z$ then leads to 
\begin{equation}
\label{eq:first_order_deriv}
\left( \bm{I} - \operatorname{diag}(\bm{z})\bm{J}_{\bm{G}}(\bm{H}) \right) \bm J_{H}(\bm z) = \operatorname{diag}(\bm{G}(\bm{H})), 
\end{equation}
or 
\begin{equation}
\bm J_{H}(\bm z) = \left( \bm{I} - \operatorname{diag}(\bm{z})\bm{J}_{\bm{G}}(\bm{H}) \right) ^{-1} \operatorname{diag}(\bm{G}(\bm{H})).
\end{equation}
The regularity of $\bm{I} - \operatorname{diag}(\bm{z})\bm{J}_{\bm{G}}(\bm{H})$ was discussed in the proof of Proposition 3.1. Therefore, as long as $|\bm z|< \bm r^\#$, the first-order derivative is finite, and it follows that $\bm H(\bm z)$ is analytic in this region. 

We can confirm this by iterative differentiation. Briefly, considering the $m$th-order derivative of $\bm H(\bm z )$ that can be derived from iterative differentiation of $\bm{H}(\bm{z}) = \operatorname{diag}(\bm{z})\bm{G}(\bm{H}(\bm{z}))$ with respect to an arbitrary sequence of variables $z_{l_1}, z_{l_2}, \ldots, z_{l_m}$, by placing only the terms that have $ \left [ \frac{\partial^{m} \bm H}{\partial z_{l_1} \ldots \partial z_{l_m}}\right] \in \mathbb{C}^n$ on the left hand side, we have that
\begin{equation}
\label{eq:higher_order_deriv}
\left( \bm{I} - \operatorname{diag}(\bm{z})\bm{J}_{\bm{G}}(\bm{H}) \right) \left [ \frac{\partial^{m} \bm H}{\partial z_{l_1} \ldots \partial z_{l_m}}\right] = \bm R^{(m-1)}(\bm z), 
\end{equation}
where $\bm R^{(m-1)}(\bm z) \in \mathbb{C}^n$ denotes a vector consisting of terms with lower-order derivatives of $\bm H(\bm z)$ and derivatives of $\bm G(\bm z)$. This essentially means that $\bm H(\bm z)$ is analytic, or that the derivatives of $\bm H(\bm z)$ are finite and well-defined in $|\bm z|< \bm r^\#$. 

%%%
%%%
\section{Details on the numerical framework for calculation of the final size distribution} 
\label{supp:implementation}

\subsection{Cauchy integral calculation}
The evaluation of PGF coefficients by Cauchy integrals has previously been described in epidemiological contexts \citep{Miller2018PGFprimer, Roberts2023EthicalControl_sciadv}. After choosing $\Gamma_{\bm{z}}$, in the main text, we evaluated the integrand of the Cauchy coefficient formula on multidimensional grids on $\Gamma_{\bm{z}}$ using DFT. As an example, for the two-dimensional cases we consider later, the grids are 
\begin{equation}
\bm{z}(l_{1},l_{2};r_1, r_2)=(r_{1}e^{2\pi \mathrm{i}\frac{l_{1}}{N}},r_{2}e^{2\pi \mathrm{i}\frac{l_{2}}{N}}), \quad l_{1}, l_{2}=0,...,N-1,
\end{equation}
and the Cauchy integral can be approximated as 
\begin{align}
\label{eq:coef_dft}
f^{(i)}(d_{1},d_{2}) &\approx \frac{1}{N^{2}}\sum_{l_{1},l_{2}=0}^{N-1}\frac{h_{i}(\bm{z}(l_{1},l_{2};r_1, r_2))}{r_{1}^{d_{1}}r_{2}^{d_{2}}}\exp\left(-\frac{2\pi \mathrm{i}}{N}(d_{1}l_{1}+d_{2}l_{2})\right).
\end{align}
In practice, we set the number of grids to $N=max(2^5, 2^{(\lceil \log_2(d_{\max}) \rceil +1)})$, where $d_{\max}$ is the maximum degree in the dataset; this is a simple rule aligning with general recommendations to reduce aliasing errors while maintaining computational efficiency \citep{trefethen2014trapezoidal, cooley1965fft}. 
\subsection{Solving the final size equation on the contour}
In the main text, we numerically solved $\bm{F}_{\bm{z}}(\bm{h})=\bm{0}$ by minimizing the scalar function $\psi_{\bm{z}}(\bm{h})= \| \bm{F}_{\bm{z}}(\bm{h}) \|^{2}_{2}$, or the product of $\bm{F}_{\bm{z}}(\bm{h})$ and its conjugate transpose (note that $\psi_{\bm{z}}(\bm{h})\ge0$ by definition). Because the argument in Proposition 3.1 ensures the regularity of the Jacobian matrix $\bm{J}_{\bm{F}_{\bm{z}}}(\bm{h})= \bm I - \operatorname{diag}(\bm z)\bm J_{\bm G}(\bm h)$ of $\bm{F}_{\bm{z}}$ when $|\bm{h}|\le \bm{r}^{\#}$, we may choose a vector $\bm{\Delta}(\bm{h})=-\bm{J}_{\bm{F}_{\bm{z}}}^{-1}(\bm{h})\bm{F}_{\bm{z}}(\bm{h})$. The definition of $\bm{\Delta}(\bm{h})$, for small $\alpha>0$ means that $\psi_{\bm{z}}(\bm{h}+\alpha\bm{\Delta}(\bm{h}))-\psi_{\bm{z}}(\bm{h}) \approx -2\alpha\psi_{\bm{z}}(\bm{h})$, and by letting $\alpha \rightarrow0$, the directional differentiation can be written as 
\begin{equation}
\frac{d}{d\alpha}\psi_{\bm{z}}(\bm{h}+\alpha\bm{\Delta}(\bm{h}))|_{\alpha=0}=-2\psi_{\bm{z}}(\bm{h}).
\end{equation}
As long as $\psi_{\bm{z}}(\bm{h})>0$, it follows that $\frac{d}{d\alpha}\psi_{\bm{z}}(\bm{h}+\alpha\bm{\Delta}(\bm{h}))|_{\alpha=0}<0$. Thus, we may compose an arbitrary sequence $\{\bm{h}^{(k)}\}$, $k=0,1,2,\dots$ by Newton steps as follows:
\begin{equation}
\bm{h}\mapsto \bm{h}+\alpha\bm{\Delta}(\bm{h}), \quad \bm{\Delta}(\bm{h})=-\bm{J}_{\bm{F}_{\bm{z}}}^{-1}(\bm{h})\bm{F}_{\bm{z}}(\bm{h}),
\end{equation}
where $\bm{h}^{(0)}$ and $\alpha\in (0, 1]$ are chosen such that $|\bm{h}^{(k)}|<\bm{r}^{\#}$ and $\psi_{\bm{z}}(\bm{h}+\alpha\bm{\Delta}(\bm{h}))<\psi_{\bm{z}}(\bm{h})$ for all $k\ge0$. For simplicity, we can start the line search from $\alpha=1$, and iterate the backtracking by $\alpha\mapsto\frac{\alpha}{2}$ up to five times; if $|\bm{h}^{(k)}|<\bm{r}^{\#}$ and $\psi_{\bm{z}}(\bm{h}+\alpha\bm{\Delta}(\bm{h}))<\psi_{\bm{z}}(\bm{h})$ cannot be satisfied within five steps, we simply switch to a Picard step $\bm{h}\mapsto \bm{T}_{\bm{z}}(\bm{h})$. Because the sequence composed in this way converges to a unique solution for every $\bm{z}$ on $\Gamma_{\bm{z}}$, as discussed in Proposition 3.1, we simply design the algorithm to start from $\bm{h}^{(0)}=\bm{0}$. 

\section{Numerical approach to ensure the validity of applying the Lagrange--Good formula}
\label{supp:LG_validity}

As described in the main text, the change-of-variables $\,\bm z \mapsto \bm h\,$ involved in the Lagrange--Good Cauchy integral for the final size of multi-type GWPs is
\begin{equation}
\label{eq:z_of_h}
z_i \;=\; \frac{h_i}{G^{(i)}(\bm h)}, \qquad i=1,\dots,n,
\end{equation}
where $G^{(i)}(\bm h)$ is the offspring PGF of type $i$ evaluated at $\bm h$: 
\begin{equation}
\label{eq:Gi_NB_form}
G^{(i)}(\bm h)
=\mathrm{denom}_i(\bm h)^{-k},
\qquad
\mathrm{denom}_i(\bm h)
=1+\frac{1}{k}\sum_{j=1}^n K_{ij}\left(1- h_j\right).
\end{equation}
The Jacobian matrix that accompanies this change of variables is
\[
\bm J_{\bm z \rightarrow \bm h} (\bm h)\;=\; \left[ \frac{\partial z_i}{\partial h_j} \right], 
\]
where
\begin{equation}
\label{eq:J_factorization}
\frac{\partial z_i}{\partial h_j}
=\frac{1}{G^{(i)}(\bm h)}
\left(
\delta_{ij} - \frac{h_i}{G^{(i)}(\bm h)}\frac{\partial G^{(i)}(\bm h)}{\partial h_j}
\right).
\end{equation}
We may factorize $\bm J_{\bm z \rightarrow \bm h} (\bm h)$ as
\begin{equation}
\label{eq:J_core}
\bm J_{\bm z \rightarrow \bm h} (\bm h) \;=\; \mathrm{diag}\!\left(\frac{1}{G^{(1)}(\bm h)},\dots,\frac{1}{G^{(n)}(\bm h)}\right)\,
\bm A(\bm h),
\qquad
A_{ij}(\bm h) \;=\; \delta_{ij} - \frac{h_i}{G^{(i)}(\bm h)}\frac{\partial G^{(i)}(\bm h)}{\partial h_j}.
\end{equation}
Therefore,
\[
\det\left(\bm J_{\bm z \rightarrow \bm h} (\bm h)\right)\neq 0
\quad\Longleftrightarrow\quad
\left(\prod_{i=1}^n G^{(i)}(\bm h)\neq 0\right)\ \text{and}\ \det\left(\bm A(\bm h) \right)\neq 0.
\]
Thus, for the numerical calculation of Lagrange--Good Cauchy integrals, we need to choose an integration contour $\Gamma_{\bm h}$ such that this condition is satisfied.  In practice, extreme values of $|\det \left( \bm J(\bm h) \right)|$ may lead to unstable numerical evaluation. Therefore, with a two-type case as an example, we select the polyradii $\bm r=(r_1,r_2)$ of 
\[
\Gamma_{\bm h} \;=\; C_{h_1}(r_1)\times C_{h_2}(r_2),
\qquad
h_\ell=r_\ell e^{i\theta_\ell},\ \theta_\ell\in[0,2\pi),
\]
as follows. Let $\bm q=(q_1,q_2)$ be the extinction probability vector (smallest real solution of $\bm q=\bm G(\bm q)$). Starting from the initial contour radii given by
\begin{equation}
\label{eq:rad_init}
r_{\ell}^{(0)}=\min\{(1-\varepsilon_{\mathrm{rad}})q_\ell,\ r_{\max}\},
\qquad
\varepsilon_{\mathrm{rad}}=10^{-2},\ \ r_{\max}=0.95,
\end{equation}
we then numerically approximate
\[
m(\bm r)\;=\;\min_{\bm h\in \Gamma_{\bm h}} |\det \left( \bm A(\bm h) \right)|
\]
for parameters  $(t,\theta_1,\theta_2)$ with
\begin{equation}
\label{eq:h_param}
\bm{h} = (t\,r_1^{(0)}e^{i\theta_1},t\,r_2^{(0)}e^{i\theta_2}),
\qquad
t\in[10^{-2},1],\ \ \theta_1,\theta_2\in[0,2\pi],
\end{equation}
under the constraint 
\begin{equation}
|\mathrm{denom}_i(\bm h)|>10^{-5}.
\end{equation}
Given the resulting approximate minimum $\widehat{m}(\bm r)$, we accept $\bm r$ if $\widehat{m}(\bm r) > \tau_{\det}$, where $\tau_{\det}=10^{-2}$. If the condition fails, we simply shrink the radius vector multiplicatively:
\begin{equation}
\bm r \leftarrow 0.9 \times\,\bm r
\end{equation}
and repeat this process. The accepted radii are stored for each scenario.

%%%
%%%
%%%
\section{Simulation of multi-type cluster data}
\label{supp:sim_data}

We generated simulated cluster data from a two-type Galton--Watson branching process.
For a type-$i \in \{1,2\}$ infectious individual, the numbers of type-1 and type-2 secondary cases $(X_{i1},X_{i2})$ follow a negative multinomial offspring distribution with a common dispersion parameter $k>0$ and mean offspring matrix $\bm K=\left[ (K_{ij})\right]$. Equivalently, conditional on the total number of secondary cases $X_{i\cdot}=X_{i1}+X_{i2}$, we draw $X_{i\cdot}\sim\mathrm{NegBin}(\text{mean}=\sum_{j}K_{ij},\text{size}=k)$, and then allocate secondary cases to types via a multinomial distribution with probabilities $K_{ij}/\sum_{j}K_{ij}$.

For each scenario, we simulated $n_1=20$ independent clusters with index type 1 and $n_2=20$ independent clusters with index type 2. Each cluster was simulated generation-by-generation starting from a single index case of the specified type, and the final size was recorded as $(N_1,N_2)$ including the index case.
The simulation was stopped when the process became extinct (no infectious individuals remained). 

%%%%%
%%%%%

\section{MCMC convergence diagnostics}
\label{supp:sec:mcmc}

Figure \ref{fig:mcmc_trace} displays the trace plots and density estimates, Figure \ref{fig:prior_posterior} displays densities of prior and posterior distributions, and Figure \ref{fig:corr_plot} displays the correlation between model parameters. In all figures, parameters 1, 2, 3, 4 denote $\log R$, $\log k$, $\operatorname{logit}(S)$, $\operatorname{logit}(\pi)$, respectively.

\begin{figure}[t]
    \centering
    \includegraphics[width=\linewidth]{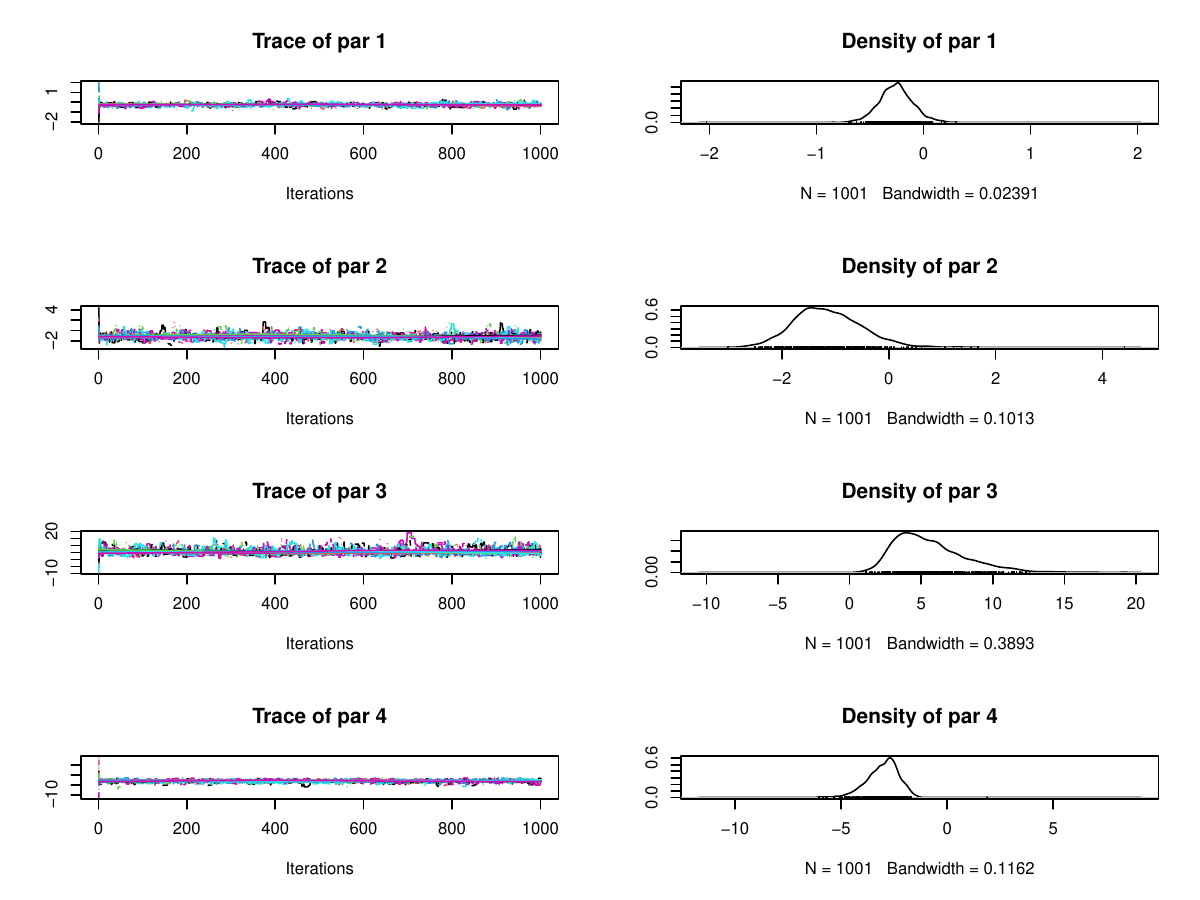}
    
    \caption{MCMC trace plots (left column) and marginal posterior density estimates (right column) for the model parameters.}
    \label{fig:mcmc_trace}
\end{figure}

\begin{figure}[t]
    \centering
    \includegraphics[width=\linewidth]{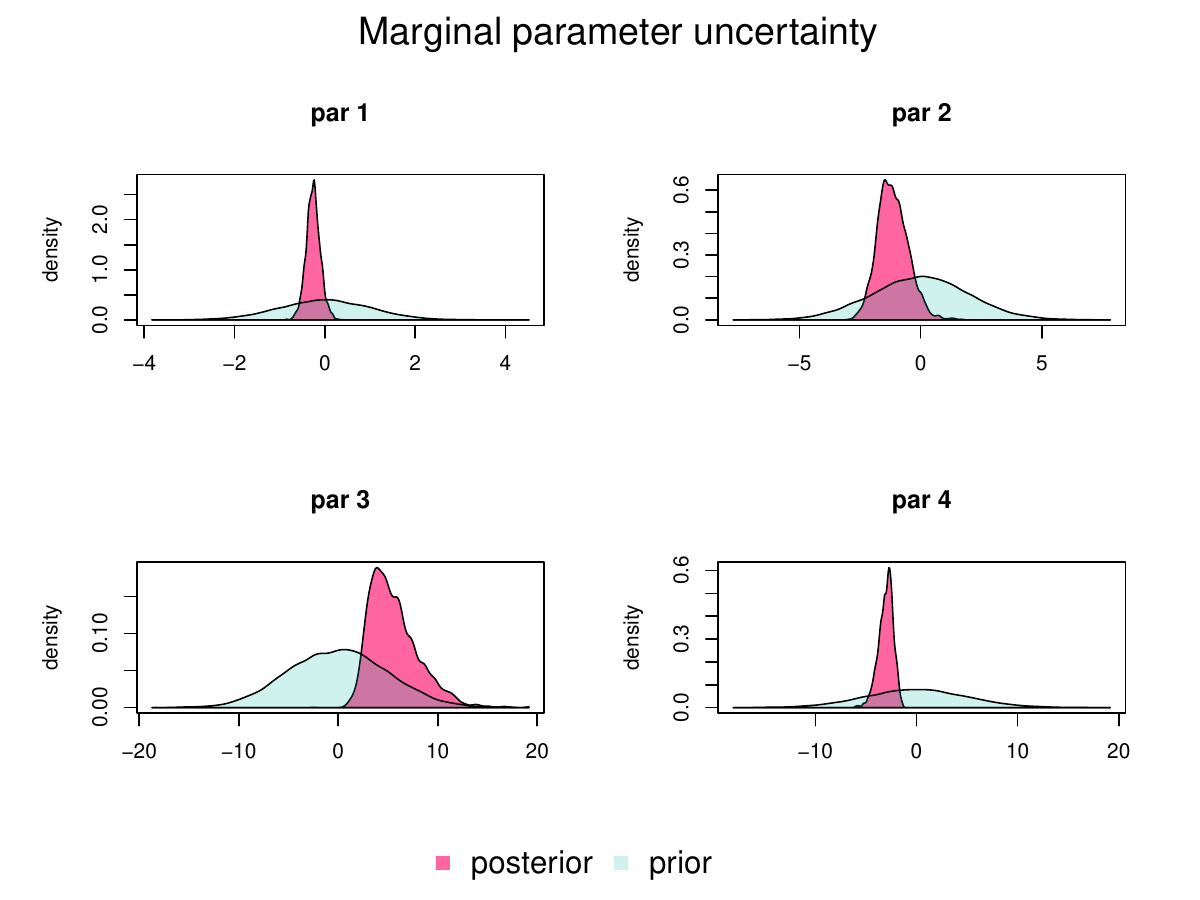}
    
    \caption{Overlay of prior and posterior densities for the model parameters. The light-blue shaded areas represent the prior distributions, whereas the red shaded areas represent the posterior distributions.}
    \label{fig:prior_posterior}
\end{figure}

\begin{figure}[t]
    \centering
    \includegraphics[width=\linewidth]{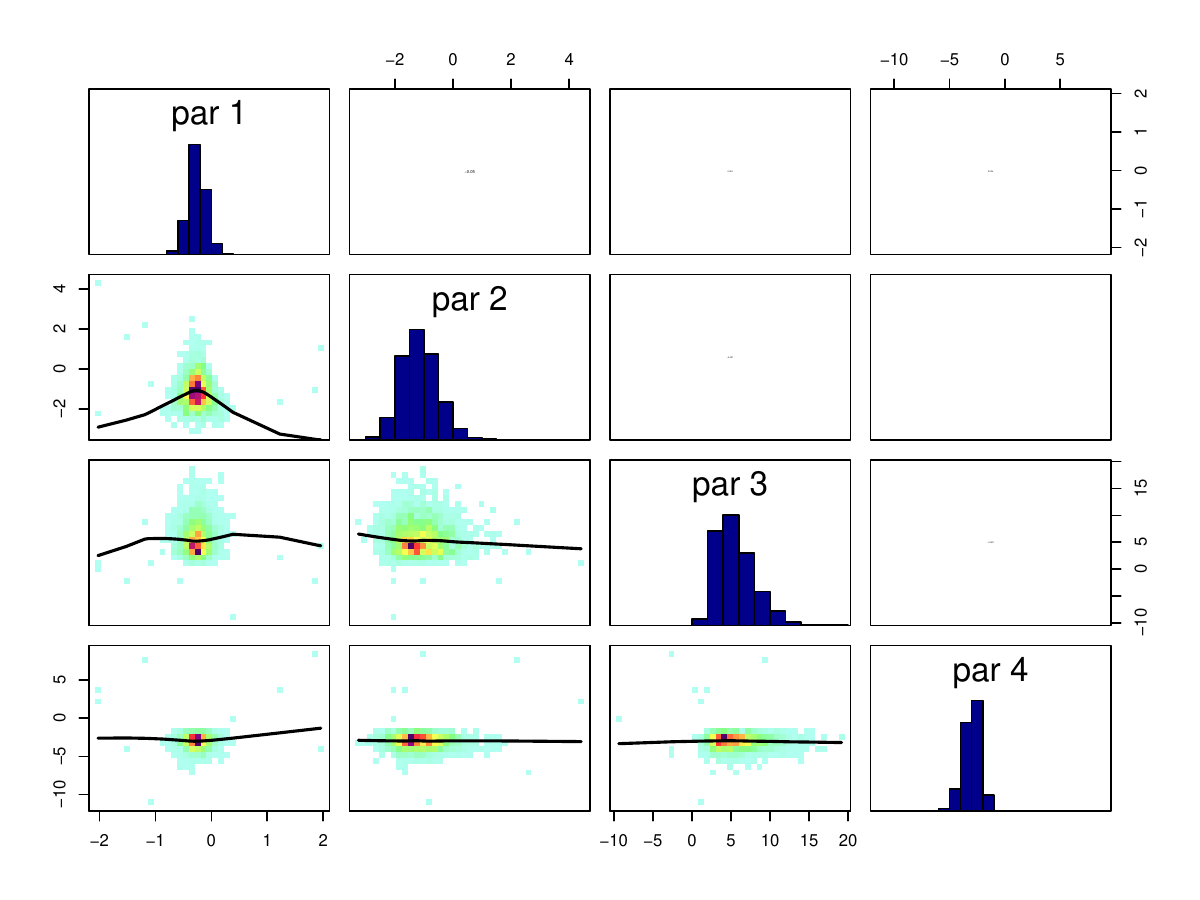}
    
    \caption{Posterior correlation plot for the MERS parameters. }
    \label{fig:corr_plot}
\end{figure}

%%%%%
%%%%%

\section{Implicit differentiation of extinction probabilities by parameters of the negative multinomial distributions}

Under the same assumptions on the offspring PGF as in Proposition 3.1, we start from the relationship $\bm{q} = \bm{G}(\bm{q})$ that the extinction probability vector $\bm{q} \in (0, 1)^n$ should satisfy. Here, $\bm{J}_{\bm{G}}(\bm{r})$ is assumed to have finite elements and is nonnegative and irreducible for $\bm r \in (0, 1]^n$.

\subsection{Differentiation by elements of the mean offspring matrix}
A small perturbation of the mean offspring matrix $\bm K= \left[ \frac{\partial G^{(i)}}{\partial z_j}\right]_{\bm z = \bm 1}$ causes a small change in $\bm q$. For simplicity, we consider a perturbation of an arbitrary $\ell$th column of the mean offspring matrix $\bm K$ (which is essentially a $\mathbb{R}^{n\times n}$ slice of the entire change in $q$) that lies in $\mathbb{R}^{n\times n \times n}$.  We denote this perturbation to $\bm{K_{\cdot \ell}} = (K_{1\ell}, \dots, K_{n\ell})^\top$, the $\ell$th column of $\bm K$, as $\bm{\Delta}_{\bm{K_{\cdot \ell}}} = (\Delta_{K_{1 \ell}}, \dots, \Delta_{K_{n\ell}})^T$. The resulting change to $\bm{q} = \bm{G}(\bm{q})$ can then be written as
\begin{equation}
 \left[  \frac{\partial q_i}{\partial K_{j\ell}}  \right]\bm{\Delta}_{\bm{K_{\cdot \ell}}}
 = \left( \left[  \frac{\partial G^{(i)}}{\partial K_{j\ell}} \right]_{\bm{z}=\bm{q}} 
 + \left[ \frac{\partial G^{(i)}}{\partial z_j} \right]_{\bm{z}=\bm{q}} \left[  \frac{\partial q_i}{\partial K_{j\ell}} \right] \right) \bm{\Delta}_{\bm{K_{\cdot \ell}}}, 
\end{equation}
which leads to 
\begin{equation}
\left( \bm{I} -  \left[ \frac{\partial G^{(i)}}{\partial z_j} \right]_{\bm{z}=\bm{q}} \right)  \left[   \frac{\partial q_i}{\partial K_{j\ell}}  \right]
 = \left[ \frac{\partial G^{(i)}}{\partial K_{j\ell}} \right]_{\bm{z}=\bm{q}} . 
\end{equation}
For $ \bm{J_G}(\bm{q}) =\left[ \frac{\partial G^{(i)}}{\partial z_j} \right]_{\bm{z}=\bm{q}}$, we know that $\rho( \bm{J_G}(q))<1$. Therefore, 
\begin{equation}
\left[  \frac{\partial q_i}{\partial K_{j\ell}} \right]
 = \left( \sum_{m=0}^\infty {\bm{J_G}(\bm{q})}^m  \right) \left[  \frac{\partial G^{(i)}}{\partial K_{j\ell}} \right]_{\bm{z}=\bm{q}}. 
\end{equation}
On the right-hand side, $\sum_{m=0}^\infty {\bm{J_G}(\bm{q})}^m$ is a strictly positive matrix because $\bm{J_G}(\bm{q})$ is irreducible. For $\left[  \frac{\partial G^{(i)}}{\partial K_{j\ell}} \right]_{\bm{z}=\bm{q}}$, we see that 
\begin{equation}
\left. \frac{\partial G^{(i)}}{\partial  K_{j\ell}} \right|_{\bm{z}=\bm{q}} =\begin{cases}
 - \left(1 -\ q_{\ell} \right)q_{i}^{1+1/k_i}<0  &  (i=j);\\
 0  &  (i \neq j).
\end{cases}
\end{equation}
In summary, $\left[ \frac{\partial q_i}{\partial K_{j\ell}}  \right]$ is a product of a positive matrix and a negative diagonal matrix. Therefore, it follows that $\frac{\partial q_i}{\partial K_{j\ell}}<0 $.

\subsection{Differentiation by overdispersion parameters}
Similarly, we may consider a small perturbation vector $\bm{\Delta}_{\bm{k}} = (\Delta_{k_1}, \dots, \Delta_{k_n})^\top$ added to $\bm{k}$. The change to $\bm{q} = \bm{G}(\bm{q})$ can be expressed as
\begin{equation}
 \left[ \frac{\partial q_i}{\partial k_j}  \right]\bm{\Delta}_{\bm{k}} 
 = \left( \left[  \frac{\partial G^{(i)}}{\partial k_j} \right]_{\bm{z}=\bm{q}} 
 + \left[ \frac{\partial G^{(i)}}{\partial z_j}  \right]_{\bm{z}=\bm{q}}\left[  \frac{\partial q_i}{\partial k_j} \right] \right) \bm{\Delta}_{\bm{k}}, 
\end{equation}
which leads to 
\begin{equation}
\left( \bm{I} -  \left[ \frac{\partial G^{(i)}}{\partial z_j}  \right]_{\bm{z}=\bm{q}} \right) \left[ \frac{\partial q_i}{\partial k_j}  \right]  
 = \left[  \frac{\partial G^{(i)}}{\partial k_j} \right]_{\bm{z}=\bm{q}}.  
\end{equation}
This can be rearranged as 
\begin{equation}
\left[  \frac{\partial q_i}{\partial k_j} \right] 
 = \left( \sum_{m=0}^\infty {\bm{J_G}(\bm{q})}^m  \right)\left[ \frac{\partial G^{(i)}}{\partial k_j} \right]_{\bm{z}=\bm{q}}. 
\end{equation}
Again, $\sum_{m=0}^\infty {\bm{J_G}(\bm{q})}^m$ is a strictly positive matrix because $ \bm{J_G}(\bm{q})$ is irreducible. For $\left[ \frac{\partial G^{(i)}}{\partial k_j} \right]_{\bm{z}=\bm{q}}$, $\frac{\partial G^{(i)}}{\partial k_j} =0$ when $i \neq j$. For $i = j$, 
\begin{equation}
\begin{split}
\left. \frac{\partial \log G^{(i)}}{\partial k_i} \right|_{\bm{z}=\bm{q}} 
&= -\log\left( 1 + \frac{1}{k_i} \sum_{m=1}^n K_{im}\left( 1 -  q_m \right) \right) + \frac{\frac{1}{k_i} \sum_{m=1}^n  K_{im}\left( 1 -  q_m \right) }{ 1 + \frac{1}{k_i} \sum_{m=1}^n K_{im}\left( 1 -  q_m \right)} \\
&=\log(q_i^{1/k_i}) + 1 - q_i^{1/k_i}.
\end{split}
\end{equation}
The final line is strictly negative ($f(x) = 1 - x + \log(x)$ is a strictly increasing function of $x \in (0, 1)$ and $\lim_{x \to 1-0} f(x) = 0$). Therefore,  $\left[  \frac{\partial G^{(i)}}{\partial k_j} \right]_{\bm{z}=\bm{q}}$ is a matrix with negative diagonal elements, and it follows that $\frac{\partial q_i}{\partial k_j} < 0$.

\begin{acks}[Acknowledgments]
Hiroshi Nishiura is also affiliated with the Center for Health Security, Graduate School of Medicine, Kyoto University.
\end{acks}

\bibliographystyle{imsart-nameyear} % Style BST file
\bibliography{references}       % Bibliography file (usually '*.bib')

\end{document}
